# Supplementary material for: RefExpo: Unveiling Software Project Structures through Advanced Dependency Graph Extraction
Source: arXiv:2407.02620 source file (2024-12-04)
Supplement: Supplementary file 1 [file appendix-evaluation.tex]

In this section, we present the evaluation of \tool\ at both micro and macro levels to assess its performance in producing dependency graphs. 
This evaluation is crucial to ensure that \tool\ accurately identifies dependencies and performs reliably in various contexts. 
The micro-level evaluation involves detailed testing with specific data suites, while the macro-level evaluation examines \tool's effectiveness across a range of popular GitHub repositories.
This approach ensures a comprehensive assessment of \tool's accuracy and robustness.

\subsection{Micro Level}

To validate \tool\ performance, we inspected two available data suites, Judge~\cite{reif-judge} and PyCG~\cite{pycg}.
Although these test suits were originally designed for constructing call graphs which are different from dependency graphs(Described in Section~\ref{app:callgraph}), we found them helpful in gauging the accuracy of \tool{}.
During the micro evaluation phase, we have run \tool\ inspection over and over and compared the outputs of it with the expected graph to fix bugs and provide the most accurate results.

Since the test suits are initially designed for call graphs, we refine them to ensure they provide accurate measurements for \tool{}. We remove all test cases that fall outside of the intended evaluation scope of \tool{}.
Nevertheless, we provided the performance analysis for both the initial and cleaned-up versions of the test suits to remove any confusion regarding the legitimacy of our evaluation.
During the cleaning process, we remove the following test cases:
\begin{itemize}
    \item \paragraphTitle{Dynamic Links}
    A complete description of why we decided to remove these links is provided in.
    \item \paragraphTitle{External References}
    We have removed all the references to external logic, such as references to \texttt{java.lang.Integer}. 
    IntelliJ is strong in reference mining and can index all the external references and even it can evaluate their internal logic and provide decompilation.
    Thus, including them in the evaluation would result in an explosion in the output size.
    Therefore, we decided to exclude them from the \tool\ evaluation scope.
\end{itemize}

Although the test cases provided in the PyCG test suite are placed in separate files, Judge test cases are defined in \texttt{.md} files.
Therefore, we process them one step further to place them in the right files and folders with small tweaks for fixing package names to be consistent with Java's required structure.
Nevertheless, both test suites are placed in our replication repository.

\paragraphTitle{Measurements}
For measuring the correctness of \tool\ evaluations we decided to use Recall.
Because originally the datasets were designed to construct a call graph we observe that \tool\ results in low accuracy.
This is because there are lots of other references in the test cases that should not be included in a call graph.
Thus, we find Recall a better indicator for the effectiveness of \tool\.
Recall is simply calculated as the ratio of the number of results correctly retrieved (True Positives) to all related results (Specified in the test suite).
\begin{equation}
    Recall = \frac{Number\ of\ correctly\ identified\ edges}{Number\ of\ all\ edges\ specified\ in\ the\ test\ suite}
\end{equation}

\paragraphTitle{Clean Up}
Table~\ref{tab:cleanup_summary} summarizes the cleanup process over Judge and PyCG test suites.
Initially, the Judge test suite contained 112 test cases and a total of 112 edges.
17 (15\%) cases were removed, resulting in the final 95 test cases.
Among those, 11 (10\%) were removed due to being an external link and six (5\%) due to being a dynamic link.

The PyCGe test suite initially contains 104 cases and a total of 223 edges.
60 (27\%) edges were removed, resulting in the final 163 edges.
Among those, 15 (7\%) were removed due to being an external link and 45(20\%) due to being a dynamic link.

\begin{table}[]
\caption{Micro test suites clean up summary}
\label{tab:cleanup_summary}
% \resizebox{\columnwidth}{!}{%
\begin{tabular}{lrr}
\hline
                   & \multicolumn{1}{l}{Judge} & \multicolumn{1}{l}{PyCG} \\ \hline
Test Cases         & 112                       & 104                      \\
Total Edges        & 112                       & 223                      \\
External Links     & 11                        & 15                       \\
Dynamic Links      & 6                         & 45                       \\
Total Clean edges  & 17                        & 60                       \\ \hline
Cleanup            & 15\%                      & 27\%                     \\ \hline
\end{tabular}%
% }
\end{table}

\paragraphTitle{Judge Test Suite}
Table~\ref{tab:judge_evaluation} summarizes \tool\ evaluation results over the Judge test suite, designed to evaluate support for different features of Java.
For 95 cases, all of the specified edges were included in the \tool\ output.
This resulted in 85\% accuracy over the initial test suite and 100\% over the cleaned version.
In both cases, the resulting accuracy is higher than the maximum accuracy reported by the Judge evaluation, which OPAL yielded as 83\%~\cite{reif-judge, reif-opal}.

\begin{tcolorbox}[colback=gray!10!white, colframe=gray!75!black, title=Micro Evaluation Java]
\tool\ yield 100\% recall during micro evaluation over the Judge test suite, which is 17\% higher than the best recall specified in the Judge evaluation.
\end{tcolorbox}

\begin{table}[]
\caption{Micro evaluation for Java over Judge test suite. `*' indicated the numbers for the cleaned data suite}
\label{tab:judge_evaluation}
\resizebox{\columnwidth}{!}{%
\begin{tabular}{lcccccc}
\hline
Feature                       & Cases & Cases*               & Corrects & Recall          & Recall* \\ \hline
Class Loading                 & 4     & 0                    & 0        & 0               & 0             \\
Dynamic Proxies               & 1     & 1                    & 1        & 1               & 1             \\
Java 8 Interface Methods      & 7     & 7                    & 7        & 1               & 1             \\
Java 8 Invoke Dynamics        & 11    & 11                   & 11       & 1               & 1             \\
JVM Calls                     & 5     & 4                    & 4        & 0.8             & 1             \\
Library                       & 5     & 4                    & 4        & 0.8             & 1             \\
Modern Reflection             & 8     & 8                    & 8        & 1               & 1             \\
Non Virtual Calls             & 5     & 5                    & 5        & 1               & 1             \\
Reflection                    & 20    & 20                   & 20       & 1               & 1             \\
Serialization                 & 14    & 7                    & 7        & 0.5             & 1             \\
Signature Polymorphic Methods & 7     & 6                    & 6        & 0.86            & 1             \\
Static Initializers           & 8     & 8                    & 8        & 1               & 1             \\
Types                         & 6     & 5                    & 5        & 0.83            & 1             \\
Unsafe                        & 7     & 7                    & 7        & 1               & 1             \\
Virtual Calls                 & 4     & 2                    & 2        & 0.5             & 1             \\ \hline
Total                         & 112   & 95                   & 95       & 0.85            & 1             \\ \hline
\end{tabular}%
}
\end{table}

\paragraphTitle{PyCG Test Suite}
Table~\ref{tab:judge_evaluation} summarizes \tool\ evaluation results over PyCG test suite.
\tool\ resulted in a 97\% recall over the cleaned test suite and 68\% over the uncleaned one.
The result is 5\% higher than the maximum accuracy yielded by PyCG which is 92\%~\cite{pycg}.
However, we should take into account that their evaluation is provided over the original version of the test suite, not the cleaned one.

\begin{tcolorbox}[colback=gray!10!white, colframe=gray!75!black, title=Micro Evaluation Python]
\tool\ yield 97\% recall during micro evaluation over the cleaned version of the PyCG test suite, which is 5\% higher than the 92\% accuracy reported for PyCG.
\end{tcolorbox}

\begin{table}[]
\caption{Micro evaluation for Python over PyCG test suite. `*' indicated the numbers for the cleaned data suite}
\label{tab:pycg_evaluation}
\resizebox{\columnwidth}{!}{%
\begin{tabular}{lcccccc}
\hline
Feature       & Tests & Edges           & Edges*       & Corrects& Recall           & Recall* \\ \hline
returns       & 4     & 12              & 8            & 8       & 0.67             & 1              \\
lambdas       & 5     & 14              & 9            & 9       & 0.64             & 1              \\
classes       & 22    & 52              & 42           & 42      & 0.81             & 1              \\
args          & 6     & 14              & 7            & 7       & 0.5              & 1              \\
decorators    & 7     & 22              & 15           & 15      & 0.68             & 1              \\
mro           & 7     & 16              & 14           & 11      & 0.69             & 0.79           \\
dicts         & 12    & 19              & 13           & 13      & 0.68             & 1              \\
exceptions    & 3     & 3               & 3            & 3       & 1                & 1              \\
dynamic       & 1     & 1               & 0            & 0       & 0                & 1              \\
imports       & 14    & 14              & 14           & 14      & 1                & 1              \\
assignments   & 4     & 15              & 15           & 15      & 1                & 1              \\
direct\_calls & 4     & 10              & 5            & 5       & 0.5              & 1              \\
builtins      & 3     & 10              & 4            & 4       & 0.4              & 1              \\
generators    & 6     & 18              & 16           & 7       & 0.39             & 0.44           \\
functions     & 4     & 4               & 4            & 4       & 1                & 1              \\
external      & 6     & 11              & 2            & 2       & 0.18             & 1              \\ \hline
Total         & 104   & 223             & 163          & 151     & 0.68             & 0.93           \\ \hline
\end{tabular}%
}
\end{table}

\subsection{Macro Level}
We compared the results of \tool\ against five existing tools over four popular GitHub repositories.

\begin{table*}[]
\caption{Macro Evalution (Python): Output comparison between \tool\, Pyan, and PyCG. (All Shared: edges that have been identified by all the tools, Two Shared: edges that are only identified by two of the tools, not the other)}
\label{tab:macroPython}
\resizebox{\textwidth}{!}{%
\begin{tabular}{lcccclccclccclccc}
\hline
Projects                      & Total Edges & All shared & Two Shared & Shared    &  & \multicolumn{3}{c}{Total}         &  & \multicolumn{3}{c}{Shared}        &  & \multicolumn{3}{c}{Unique}      \\ \cline{7-9} \cline{11-13} \cline{15-17} 
                              &             &            &            &           &  & RefExpo    & Pyan      & PyCG      &  & RefExpo   & Pyan      & PyCG      &  & RefExpo   & Pyan      & PyCG    \\ \cline{1-5} \cline{7-9} \cline{11-13} \cline{15-17} 
TheAlgorithms/Python          & 1733        & 356(21\%)  & 409(24\%)  & 765(44\%) &  & 1405(81\%) & 961(55\%) & 488(28\%) &  & 761(44\%) & 733(42\%) & 392(23\%) &  & 644(37\%) & 228(13\%) & 96(6\%) \\
wting/autojump                & 566         & 96(17\%)   & 88(16\%)   & 184(33\%) &  & 487(86\%)  & 214(38\%) & 145(26\%) &  & 184(33\%) & 155(27\%) & 125(22\%) &  & 303(54\%) & 59(10\%)  & 20(4\%) \\
aboul3la/Sublist3r            & 236         & 22(9\%)    & 69(29\%)   & 91(39\%)  &  & 234(99\%)  & 34(14\%)  & 81(34\%)  &  & 91(39\%)  & 32(14\%)  & 81(34\%)  &  & 143(61\%) & 2(1\%)    & 0(0\%)  \\
oarriaga/face\_classification & 191         & 19(10\%)   & 25(13\%)   & 44(23\%)  &  & 182(95\%)  & 44(23\%)  & 28(15\%)  &  & 44(23\%)  & 44(23\%)  & 19(10\%)  &  & 138(72\%) & 0(0\%)    & 9(5\%)  \\ \hline
Average                       & 682         & 14\%       & 21\%       & 35\%      &  & 90\%       & 33\%      & 26\%      &  & 35\%      & 27\%      & 22\%      &  & 56\%      & 6\%       & 4\%     \\ \hline
\end{tabular}%
}
\end{table*}

\begin{table*}[]
\caption{Macro Evalution(Java): Output comparison between \tool\, Jarviz, Dependency Finder, and Sonargraph. (All Shared: edges that have been identified by all the tools, Two Shared: 
edges that are only identified by two of them, not the others)}
\label{tab:macroJava}
\resizebox{\textwidth}{!}{%
\begin{tabular}{lccccclcccclcccclcccc}
\hline
Projects             & Total Edges & All shared & Two Shared  & Three Shared & Shared      &  & \multicolumn{4}{c}{Totals}                             &  & \multicolumn{4}{c}{Shared}                            &  & \multicolumn{4}{c}{Unique}                    \\ \cline{8-11} \cline{13-16} \cline{18-21} 
                     &             &            &             &              &             &  & RefExpo      & Jarviz      & DF          & Sonargraph  &  & RefExpo     & Jarviz      & DF          & Sonargraph  &  & RefExpo     & Jarviz  & DF       & Sonargraph \\ \cline{1-6} \cline{8-11} \cline{13-16} \cline{18-21} 
google/guava         & 9,249       & 335(4\%)   & 3,726(40\%) & 2,650(29\%)  & 6,711(73\%) &  & 8,382(91\%)  & 4,329(47\%) & 2,200(24\%) & 4,369(47\%) &  & 6,592(71\%) & 4,302(47\%) & 1,941(21\%) & 3,907(42\%) &  & 1,790(19\%) & 27(0\%) & 259(3\%) & 462(5\%)   \\
ReactiveX/RxJava     & 10,738      & 473(4\%)   & 6,894(64\%) & -            & 7,367(69\%) &  & 10,210(95\%) & 6,969(65\%) & 1,399(13\%) & -           &  & 7,367(69\%) & 6,924(64\%) & 916(9\%)    & -           &  & 2,843(26\%) & 45(0\%) & 483(4\%) & -          \\
square/retrofit      & 712         & 36(5\%)    & 160(22\%)   & -            & 196(28\%)   &  & 657(92\%)    & 166(23\%)   & 121(17\%)   & -           &  & 193(27\%)   & 161(23\%)   & 74(10\%)    & -           &  & 464(65\%)   & 5(1\%)  & 47(7\%)  & -          \\
FastXML/jackson-core & 899         & 175(19\%)  & 90(10\%)    & 337(37\%)    & 602(67\%)   &  & 818(91\%)    & 252(28\%)   & 555(62\%)   & 563(63\%)   &  & 599(67\%)   & 241(27\%)   & 491(55\%)   & 560(62\%)   &  & 219(24\%)   & 11(1\%) & 64(7\%)  & 3(0\%)     \\ \hline
Average              & 5,400       & 8\%        & 34\%        & 48\%         & 60\%        &  & 92\%         & 41\%        & 29\%        & 55\%        &  & 59\%        & 40\%        & 24\%        & 52\%        &  & 34\%      & 1\%     & 5\%      & 3\%        \\ \hline
\end{tabular}%
}
\end{table*}

\paragraphTitle{Metrics}
To compare different tools, we create a list of the edges that the tools identify as edges of the graph, and we evaluate the overlaps.
We visualize the overlap analysis outcome by drawing Venn diagrams that show the exact number of overlaps between different tools.
Afterward, we define the ratio of unique results count to the total number of edges as a measure of the uniqueness of each tool's results.
Similarly, we define the ratio of shared and total edges.
It should be noted that all these ratios are calculated based on the total number of edges that have been identified by all the tools.
Hence, for each tool the ratio of unique edges plus the ratio of the shared edges is not equal to one but the ratio of its total edges.

\paragraphTitle{Tool Selection}
For this study, we have concentrated on evaluating tools that offer assessments for the Java and Python programming languages.
We compare the performance of \tool\ against all language-specific tools discussed in Section~\ref{app:relatedWorks}.

\paragraphTitle{Project Selection}
To remove any bias from our evaluation we tried to select popular projects from GitHub.
Initially, we used the same methodology that we have used for constructing our dataset.
During our evaluation, we never encountered any project that \tool\ can not evaluate.
However, due to limitations of other tools we needed to change our approach accordingly.

\paragraphTitle{Python.} 
Since PyCG and Pyan are only compatible with Python 3.6 and 3.7 we faced a barrier in selecting our repositories.
We observed that almost all popular GitHub projects are under active development.
Thus, they are updated and are using new technologies.
Consequently, we could not run both PyCG and Pyan over any of the most popular repositories in their current version at the time.
However, we could successfully run PyCG and Pyan over one of the older revisions of \texttt{TheAlgorithms/Python} project. 
The tools were able to provide an evaluation for the latest version of the project published before February 2019. 
This is because Python 3.8 was introduced in the same year and the developers started to integrate new language features. 

Although it is not a real production project and was developed for educational purposes, it still contains 1407 files and gained 175 starts.
Moreover, we found out we could run PyCG and Pyan over three out of five repositories evaluated in the original PyCG study.
They are substantially smaller than the projects we aimed to evaluate and are not maintained for years which makes them compatible with both tools.
Despite, their size and lack of maintenance, they gained more than 5k starts which makes them legitimate projects for evaluation.
In the end, we came up with a set of four projects described in the replication package~\footnote{\url{https://github.com/vharatian/RefExpo}, \label{tool}}, \texttt{TheAlgorithms/Python}, \texttt{wting/autojump}, \texttt{aboul3la/Sublist3r}, \texttt{oarriaga/face\_classification}.

As demonstrated in Table~\ref{tab:macroPython} and Figure~\ref{fig:results} on average \tool\ covered 90\% of the identified edges, Pyan 33\% of them, and PyCg 26\%.
Among those edges that have been covered by \tool\, 35\% of them were shared, and 56\% of them were unique.
Similarly, Pyan and PyCG yielded 27\% and 22\% of shared edges and 6\% and 4\% of unique edges.
We have observed that Pyan is the second best-performing tool regarding the ratio of shared and unique edges.
Our results show that there is a good number of edges that are identified by only two of the tools (21\%) while the majority of these edges are between \tool\ and one of the Pyan or PyCG.
Usually, the intersection area between PyCG and Pyan is below 1\% meaning that \tool\ is more agreeable compared to both of them.

\begin{tcolorbox}[colback=gray!10!white, colframe=gray!75!black, title=Macro Evaluation Results for Python]
\tool\ yield superior results regarding the unique and shared number of edges which are 50\% and 8\% higher than the next best-performing tool, Pyan. \tool\ is the most agreeable among the three tools by having more one-to-one overlaps.
\end{tcolorbox}

\textit{Java.} 
We have better options when it comes to Java evaluation since the tools are more mature and are compatible with recent Java versions.
Nevertheless, we could not pick the top most popular repositories since some of the tools only can provide evaluation for JAR files.
Still, some of the most popular repositories have their JAR file built and ready to use over Maven.
Even though one of the projects that is listed as the top repositories, Jackson, does not build into a single JAR file, we could run our evaluation over a submodule of it \texttt{jackson-core} which its JAR file is available on public repositories.
Besides, the test codes are not available in the built JAR files available in the public repositories. 
Hence, we needed to manually delete all the test files to make a fair comparison between the tools.
We further removed all the sample codes included in the repository for the same reason.
Finally, we could not configure Sonargraph on two of the projects since it was constantly crashing and we could not find the right configuration. 
However, we decided to keep the project since other tools were able to provide evaluations.
This results in four final projects described in the replication package~\footref{tool}, \texttt{google/guava}, \texttt{FastXML/jackson-core}, \texttt{ReactiveX/RxJava}, \texttt{square/retrofit}.

As demonstrated in Table~\ref{tab:macroJava} and Figure~\ref{fig:results} on average \tool\ covered 92\% of the identified edges, Jarviz 41\%, Dependency Finder 29\%, and Sonargraph 55\%.
Among those edges that have been covered by \tool\, 59\% of them were shared, and 34\% of them were unique.
Similarly, Jarviz, Dependency Finder, and Sonargraph yielded 40\%, 24\%, and 52\% of shared edges and 1\%, 5\% and 3\% of unique edges.
A full comparison of the results has been demonstrated in Figure~\ref{fig:results}
We have observed that Sonargraph is the second best-performing tool regarding the ratio of shared edges. 
Nevertheless, Dependency Finder yielded the second-best results regarding unique results.
Our results show that there is a good number of edges that are identified by only two or three of the tools (52\%) while the majority of these edges are identified by \tool{}.
Usually, the intersection areas that fall outside of \tool\ circle have a value less than 1\%.

\begin{tcolorbox}[colback=gray!10!white, colframe=gray!75!black, title=Macro Evaluation Results for Java]
\tool\ yield superior results regarding the unique and shared number of edges which are 31\% and 7\% higher than the next best-performing tools, Sonargraph and Dependency Finder. \tool\ is the most agreeable among the four tools by having more overlaps.
\end{tcolorbox}

\begin{figure*}[ht]
    \centering
    \begin{subfigure}[text]{0.33\textwidth}
        \centering
        \includegraphics[width=\textwidth]{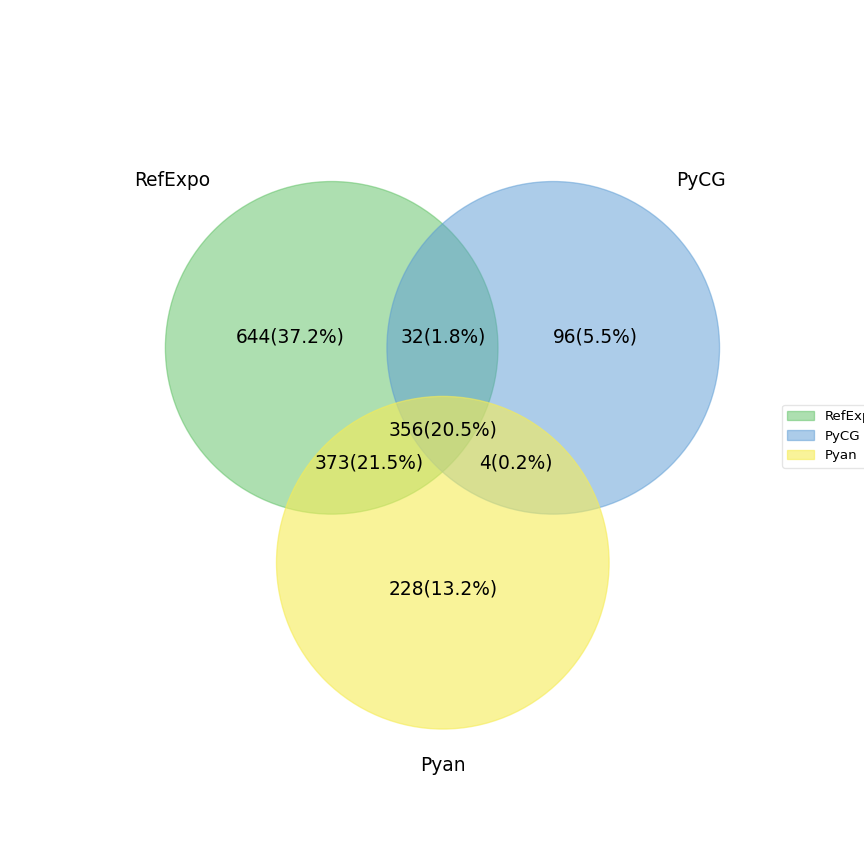}
        \caption{TheAlgorithms/Python}
        \label{fig:resultsPython}
    \end{subfigure}
    \begin{subfigure}[text]{0.33\textwidth}
        \centering
        \includegraphics[width=\textwidth]{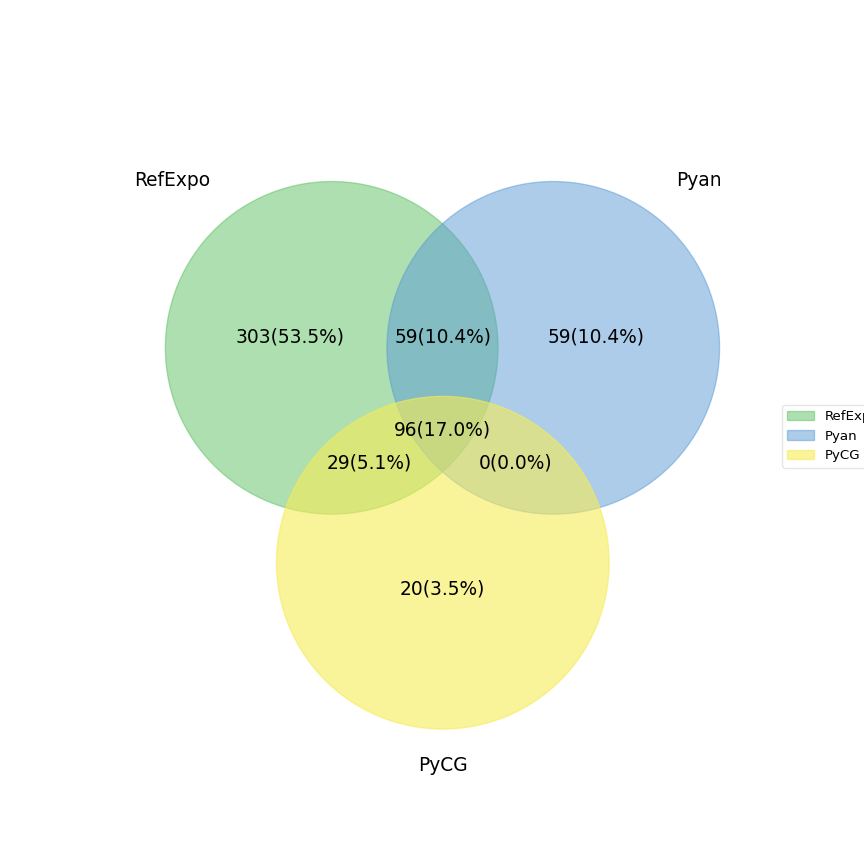}
        \caption{wting/autojump}
        \label{fig:resultsAutojump}
    \end{subfigure}
    \begin{subfigure}[text]{0.33\textwidth}
        \centering
        \includegraphics[width=\textwidth]{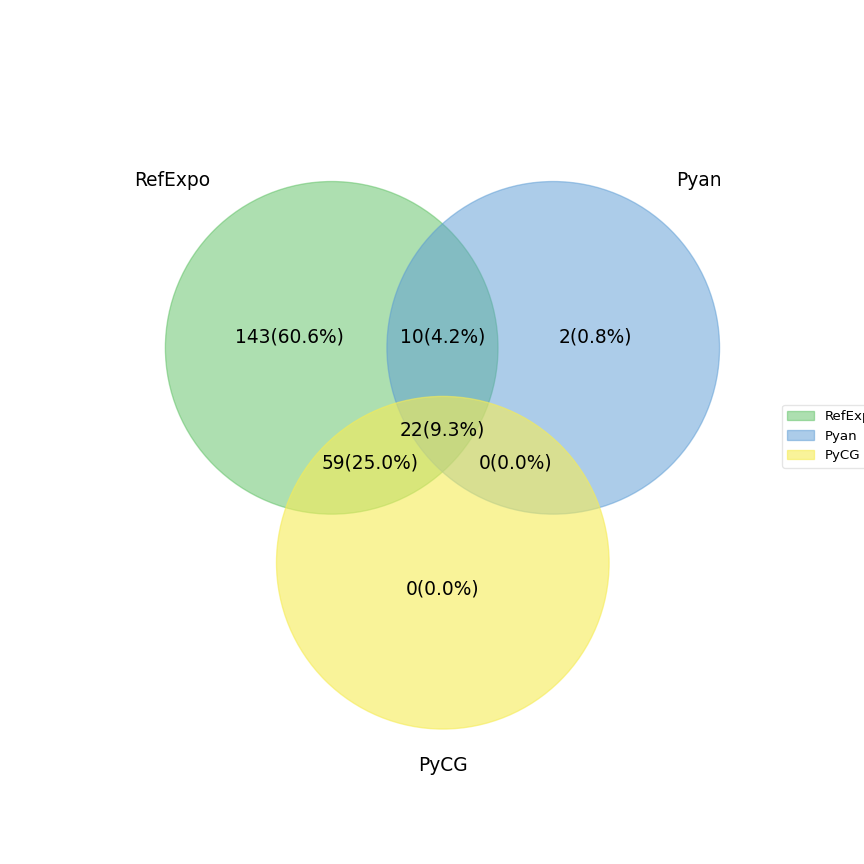}
        \caption{aboul3la/Sublist3r}
        \label{fig:resultsSublist}
    \end{subfigure}
    \begin{subfigure}[text]{0.33\textwidth}
        \centering
        \includegraphics[width=\textwidth]{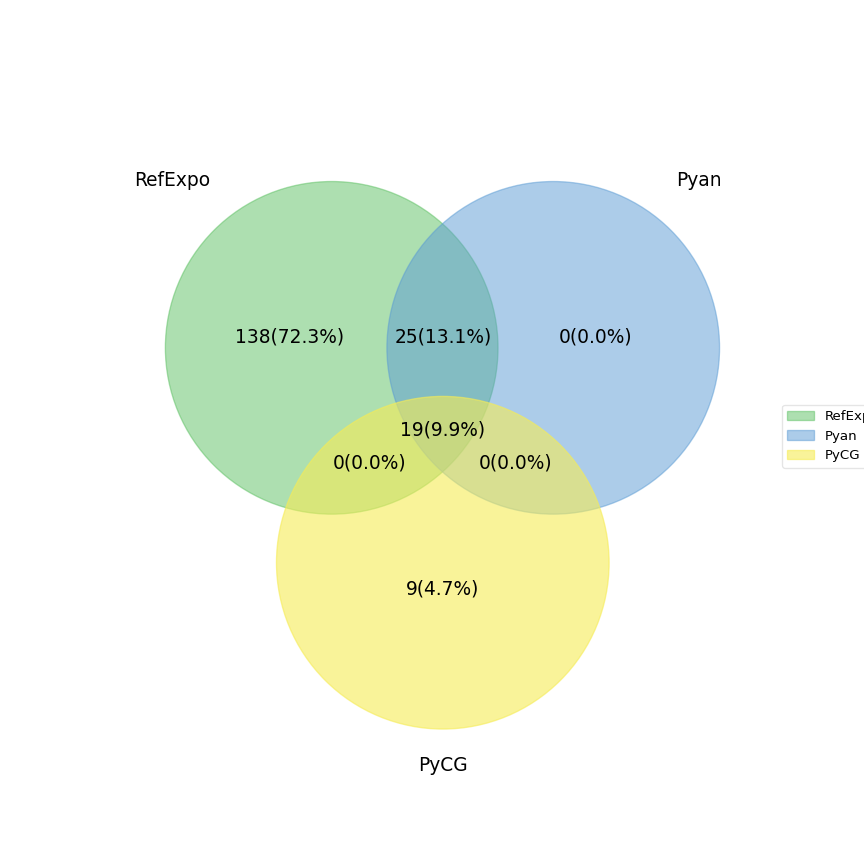}
        \caption{oarriaga/face\_classification}
        \label{fig:resultsFaceClassification}
    \end{subfigure}
    \begin{subfigure}[text]{0.33\textwidth}
        \centering
        \includegraphics[width=\textwidth]{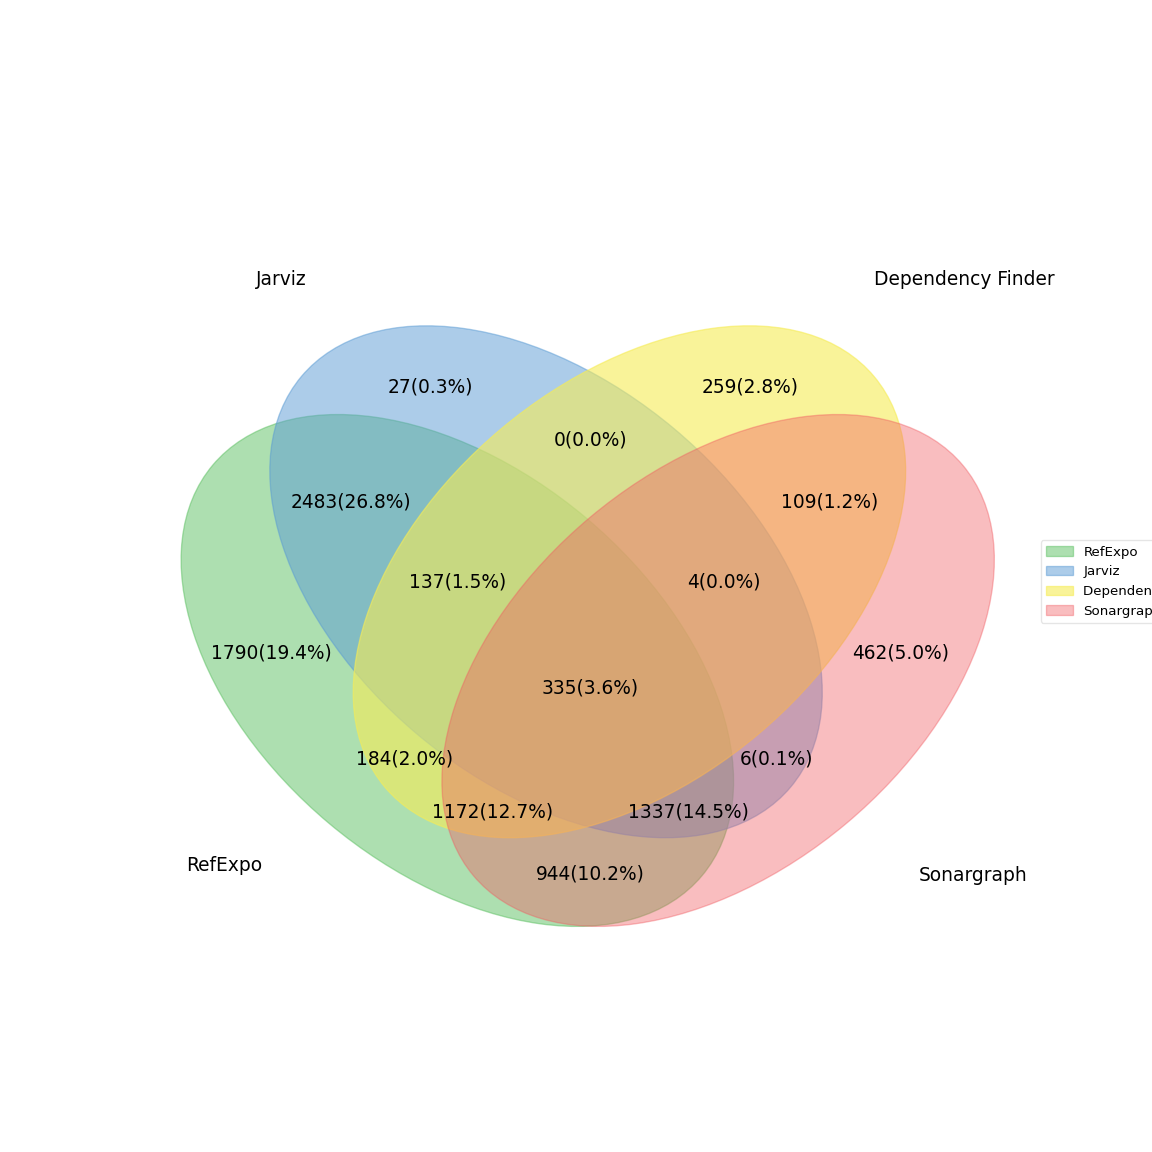}
        \caption{google/guava}
        \label{fig:resultsGuava}
    \end{subfigure}
    \begin{subfigure}[text]{0.33\textwidth}
        \centering
        \includegraphics[width=\textwidth]{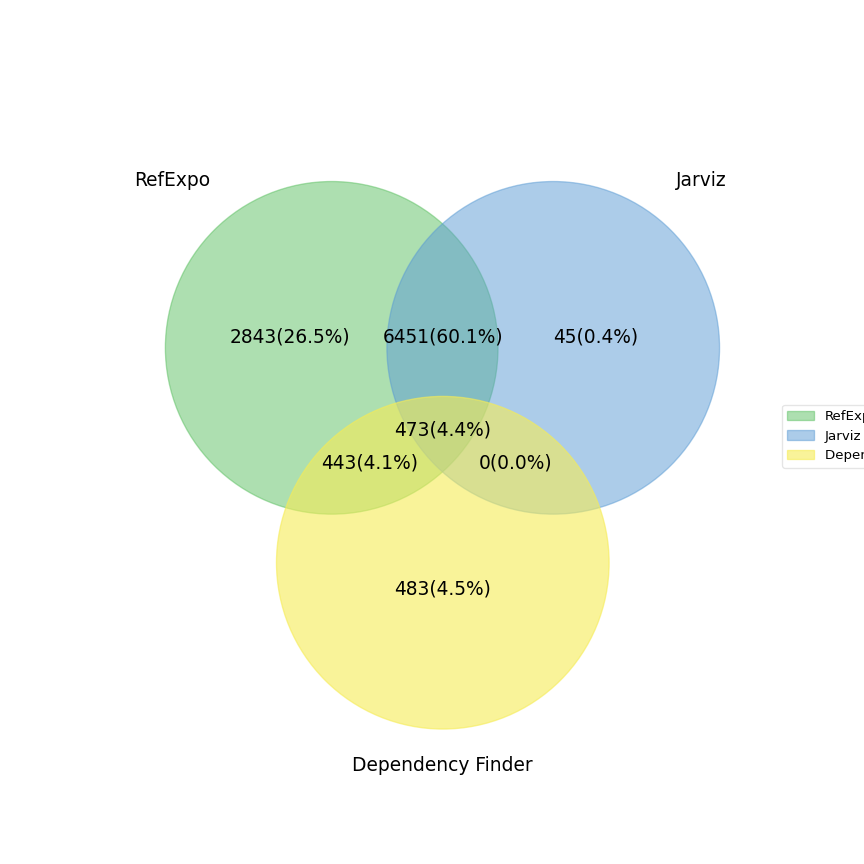}
        \caption{ReactiveX/RxJava}
        \label{fig:resultsRxjava}
    \end{subfigure}
    \begin{subfigure}[text]{0.33\textwidth}
        \centering
        \includegraphics[width=\textwidth]{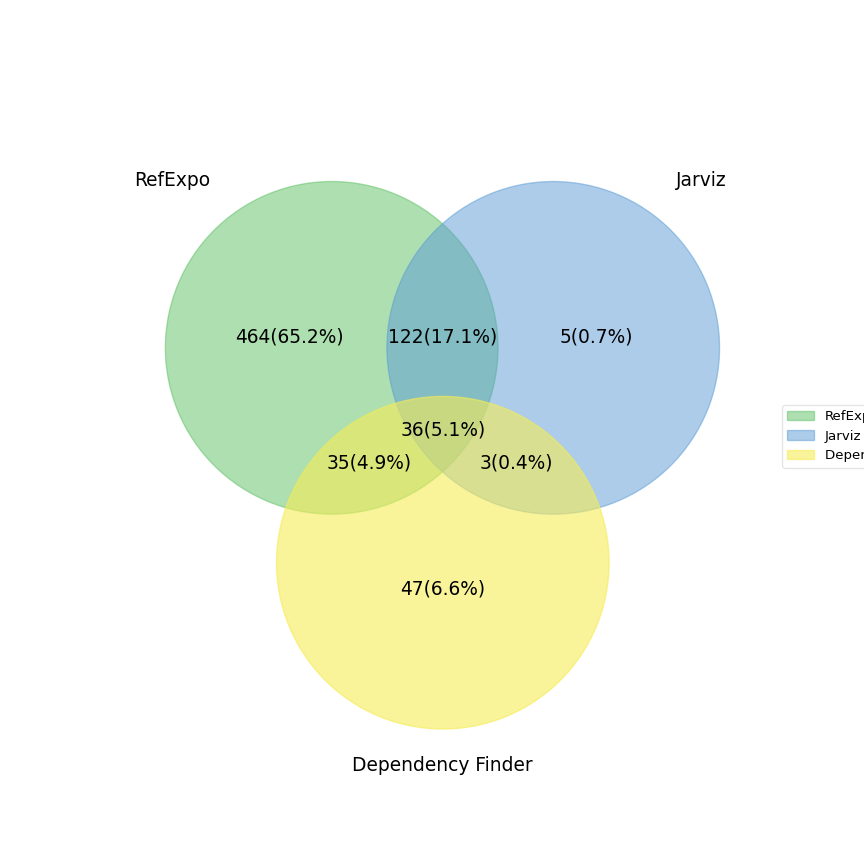}
        \caption{square/retrofit}
        \label{fig:resultsRetrofit}
    \end{subfigure}
    \begin{subfigure}[text]{0.33\textwidth}
        \centering
        \includegraphics[width=\textwidth]{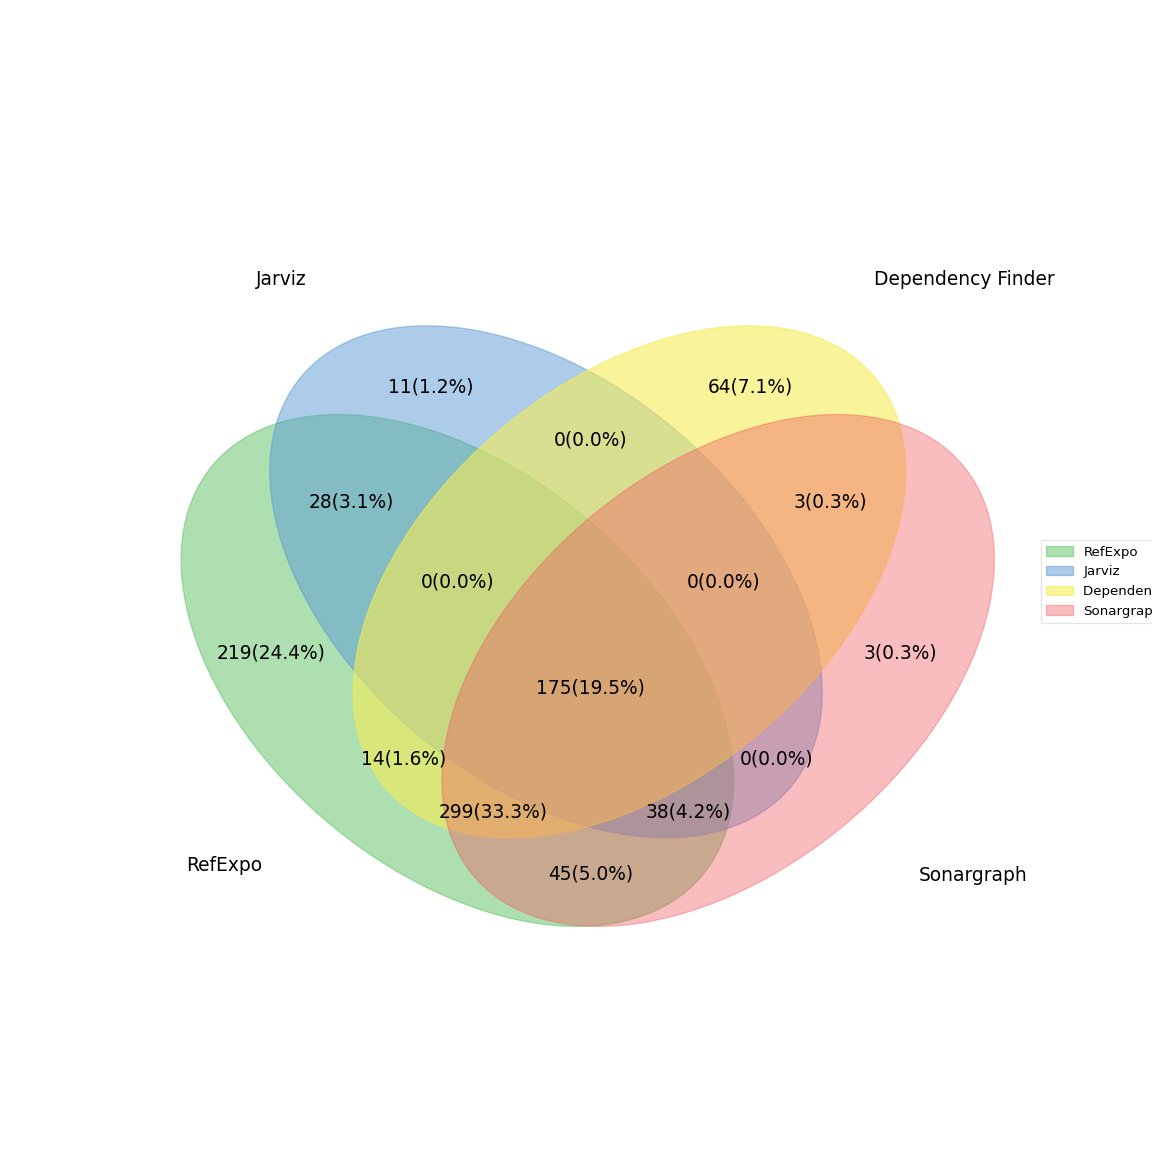}
        \caption{FastXML/jackson-core}
        \label{fig:resultsJackson}
    \end{subfigure}
    
    \caption{Macro evaluation over eight GitHub repositories, Four Java and Four Python}
    \label{fig:results}
\end{figure*}
