# Supplementary material for: RefExpo: Unveiling Software Project Structures through Advanced Dependency Graph Extraction
Source: arXiv:2407.02620 source file (2024-12-04)
Supplement: Supplementary file 2 [file appendix-summary.tex]

This appendix provides an in-depth exploration and evaluation of \tool{}, a software tool designed to generate dependency graphs from source code. 
The main goal of \tool\ is to assist researchers and experts in comprehending and managing complex codebases by identifying and visualizing the relationships and dependencies among various components.

The appendix is divided into three main sections.
Section~\ref{app:relatedWorks} to discuss the related works and the tool we compared \tool\ against. 
Section~\ref{app:callgraph} to clarify the distinctions between dependency graphs and call graphs.
And Section~\ref{app:evaluation} includes comprehensive analyses, detailing the methodologies employed, the metrics used for evaluation, and the detailed results of both micro and macro-level assessments. The aim is to provide an in-depth understanding of \tool's capabilities and reliability.
